# Supplementary material for: SHORTSTACK: Distributed, Fault-tolerant, Oblivious Data Access
Source: arXiv:2205.14281 source file (2022-06-08)
Supplement: Supplementary file 1 [file main.tex]

\PassOptionsToPackage{usenames, dvipsnames, svgnames, table}{xcolor}
\documentclass[letterpaper,twocolumn,10pt]{article}
\usepackage{usenix-2020-09}

\newif \ifcomments \commentstrue
% \commentsfalse

\newif \iffullversion \fullversiontrue
\fullversionfalse

\input{../tex/packages}
\input{../tex/envirs}
\input{../tex/defs}
\usepackage{graphicx}
\usepackage{epstopdf}
\usepackage[export]{adjustbox}
\epstopdfsetup{update}

\makeatletter
\newcommand{\customlabel}[2]{%
   \protected@write \@auxout {}{\string \newlabel {#1}{{#2}{\thepage}{#2}{#1}{}} }%
   \hypertarget{#1}{}
}
\makeatother

\begin{document}

%don't want date printed
\date{}

% make title bold and 14 pt font (Latex default is non-bold, 16 pt)
\title{Supplementary Material}

% %for single author (just remove % characters)
\author{Paper \#381
% % {\rm Kushal Babel}\\
% % babel@cs.cornell.edu
% % \and
% % {\rm Midhul Vuppalapati}\\
% % midhul@cs.cornell.edu
% % copy the following lines to add more authors
% % \and
% % {\rm Name}\\
% %Name Institution
} % end author

\maketitle

\begin{sloppypar}
    \input{appendix}
    \input{appendix2}
    {
    \balance
    \bibliographystyle{plain}
    \bibliography{../bib/citations}
    \appendix
    }
\end{sloppypar}

\end{document}
